# Supplementary material for: Rotation-Agnostic Image Representation Learning for Digital Pathology
Source: arXiv:2311.08359 source file (2024-03-12)

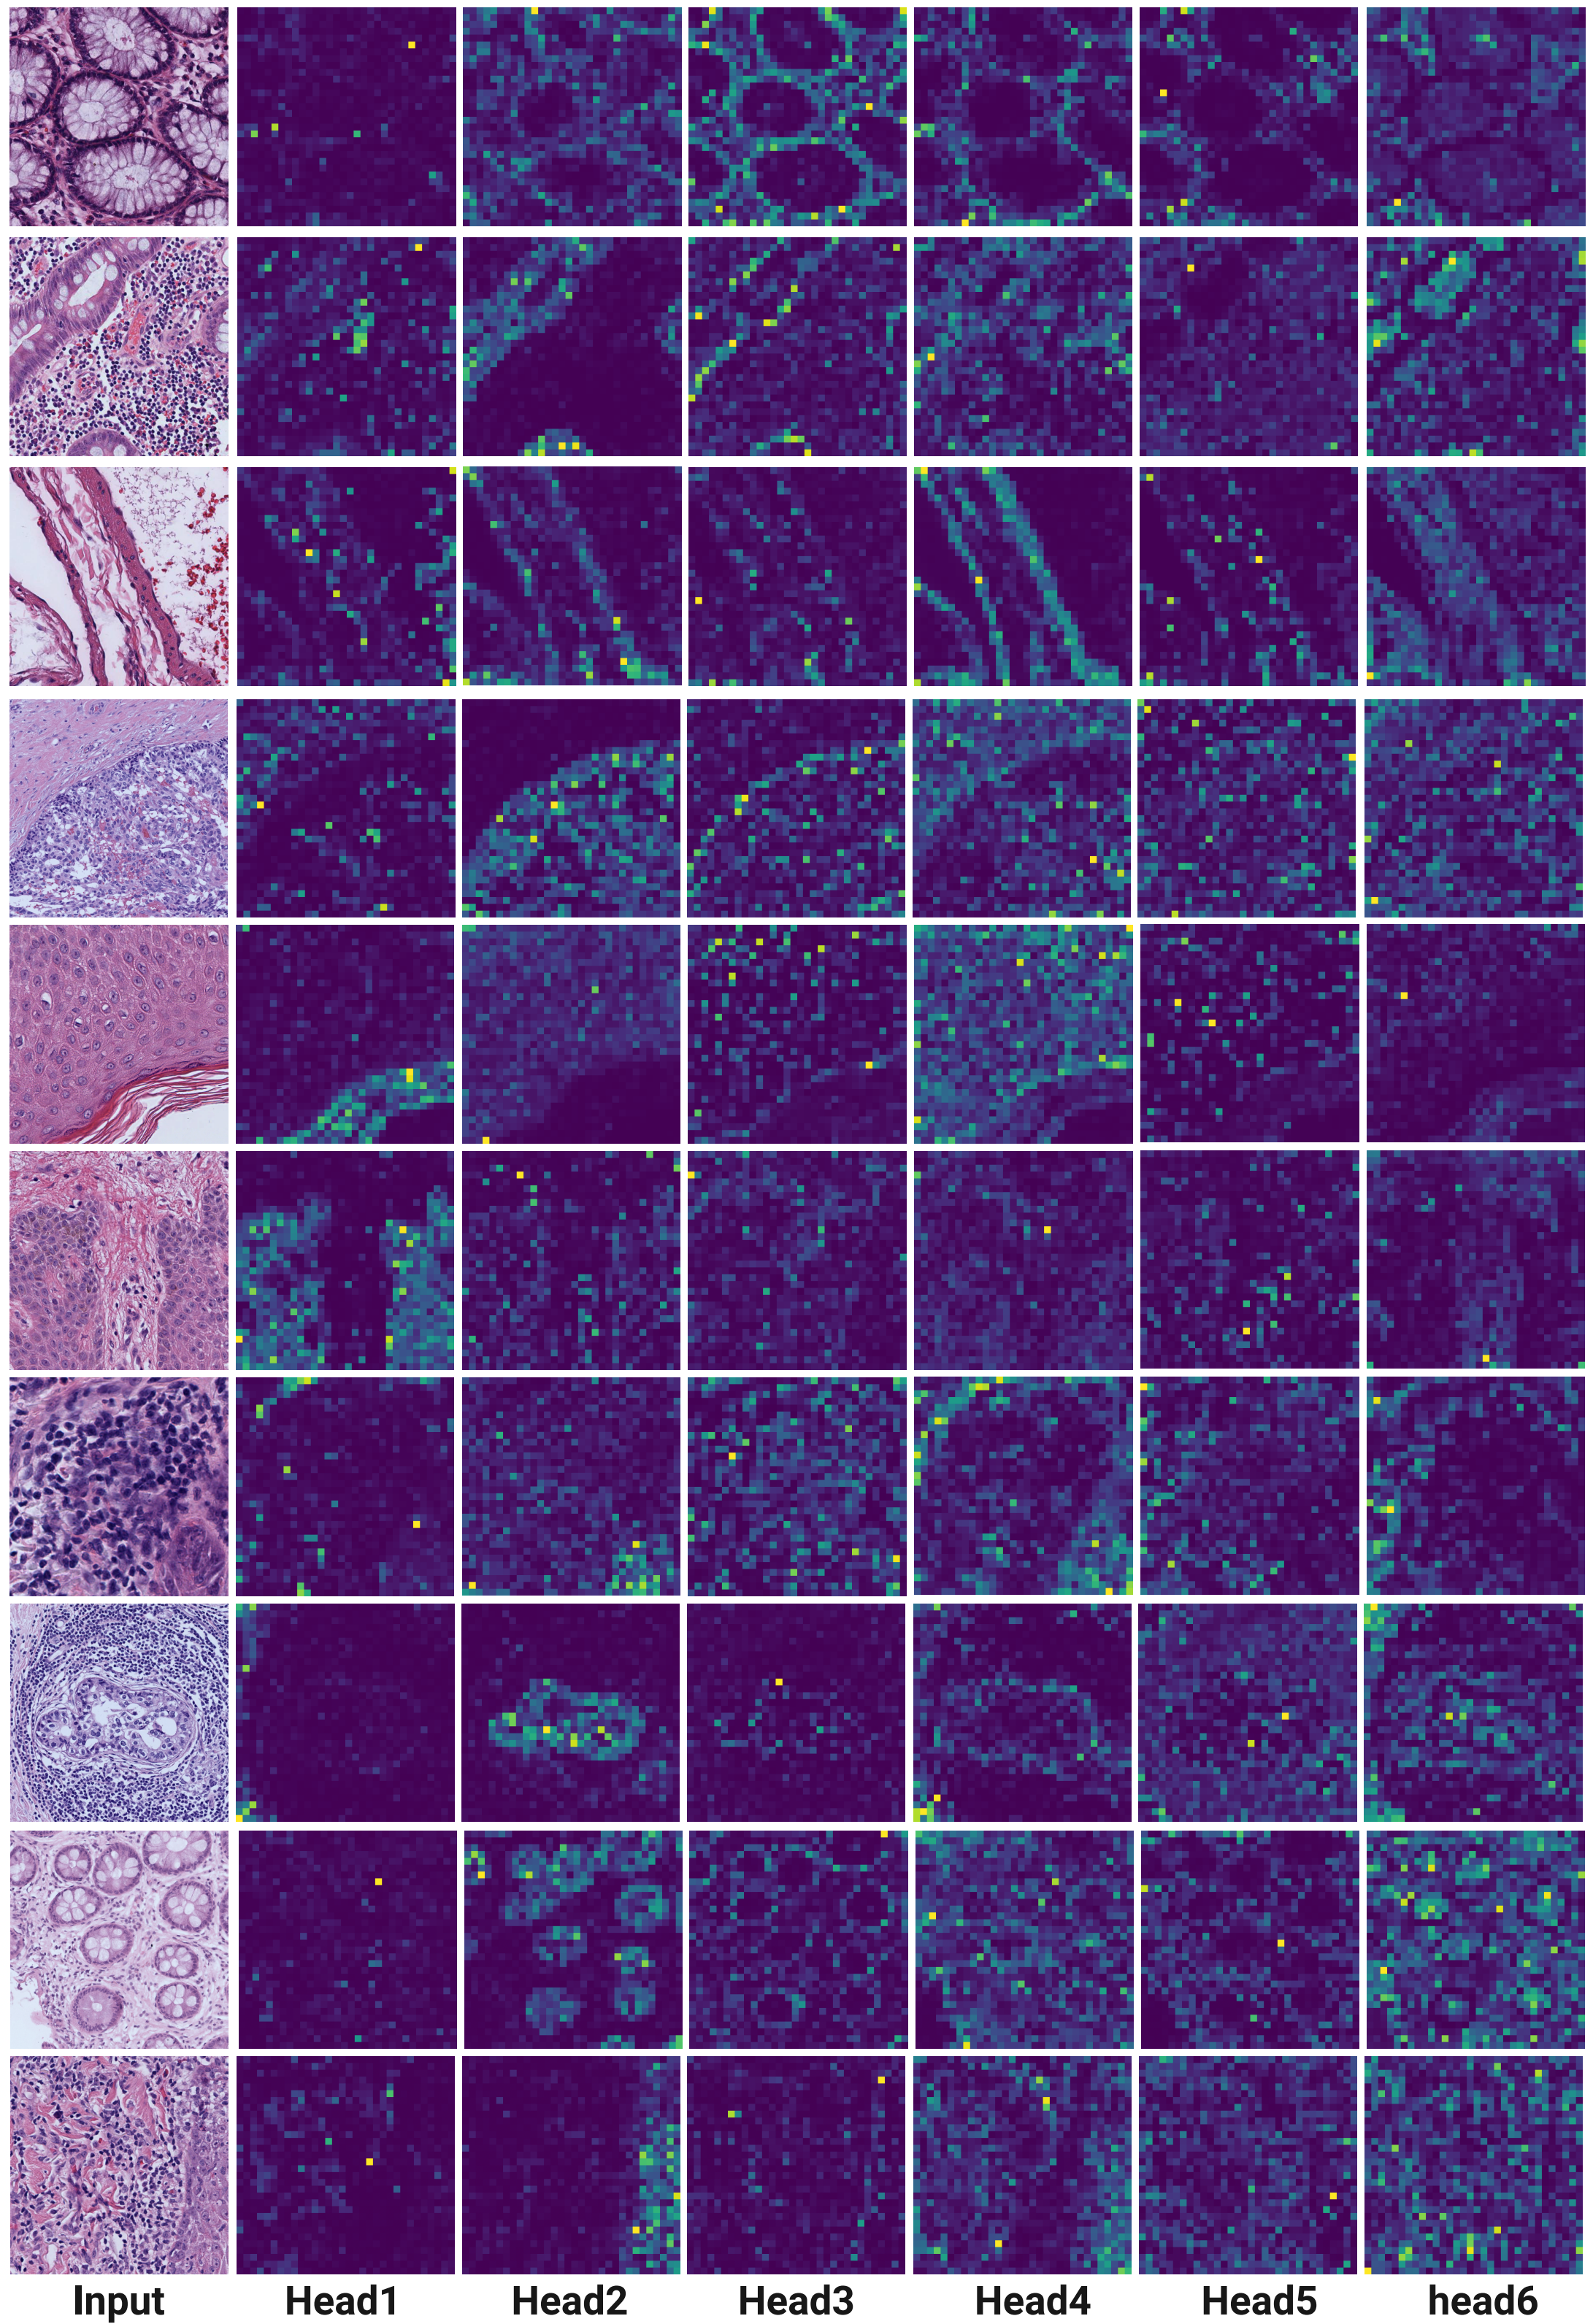

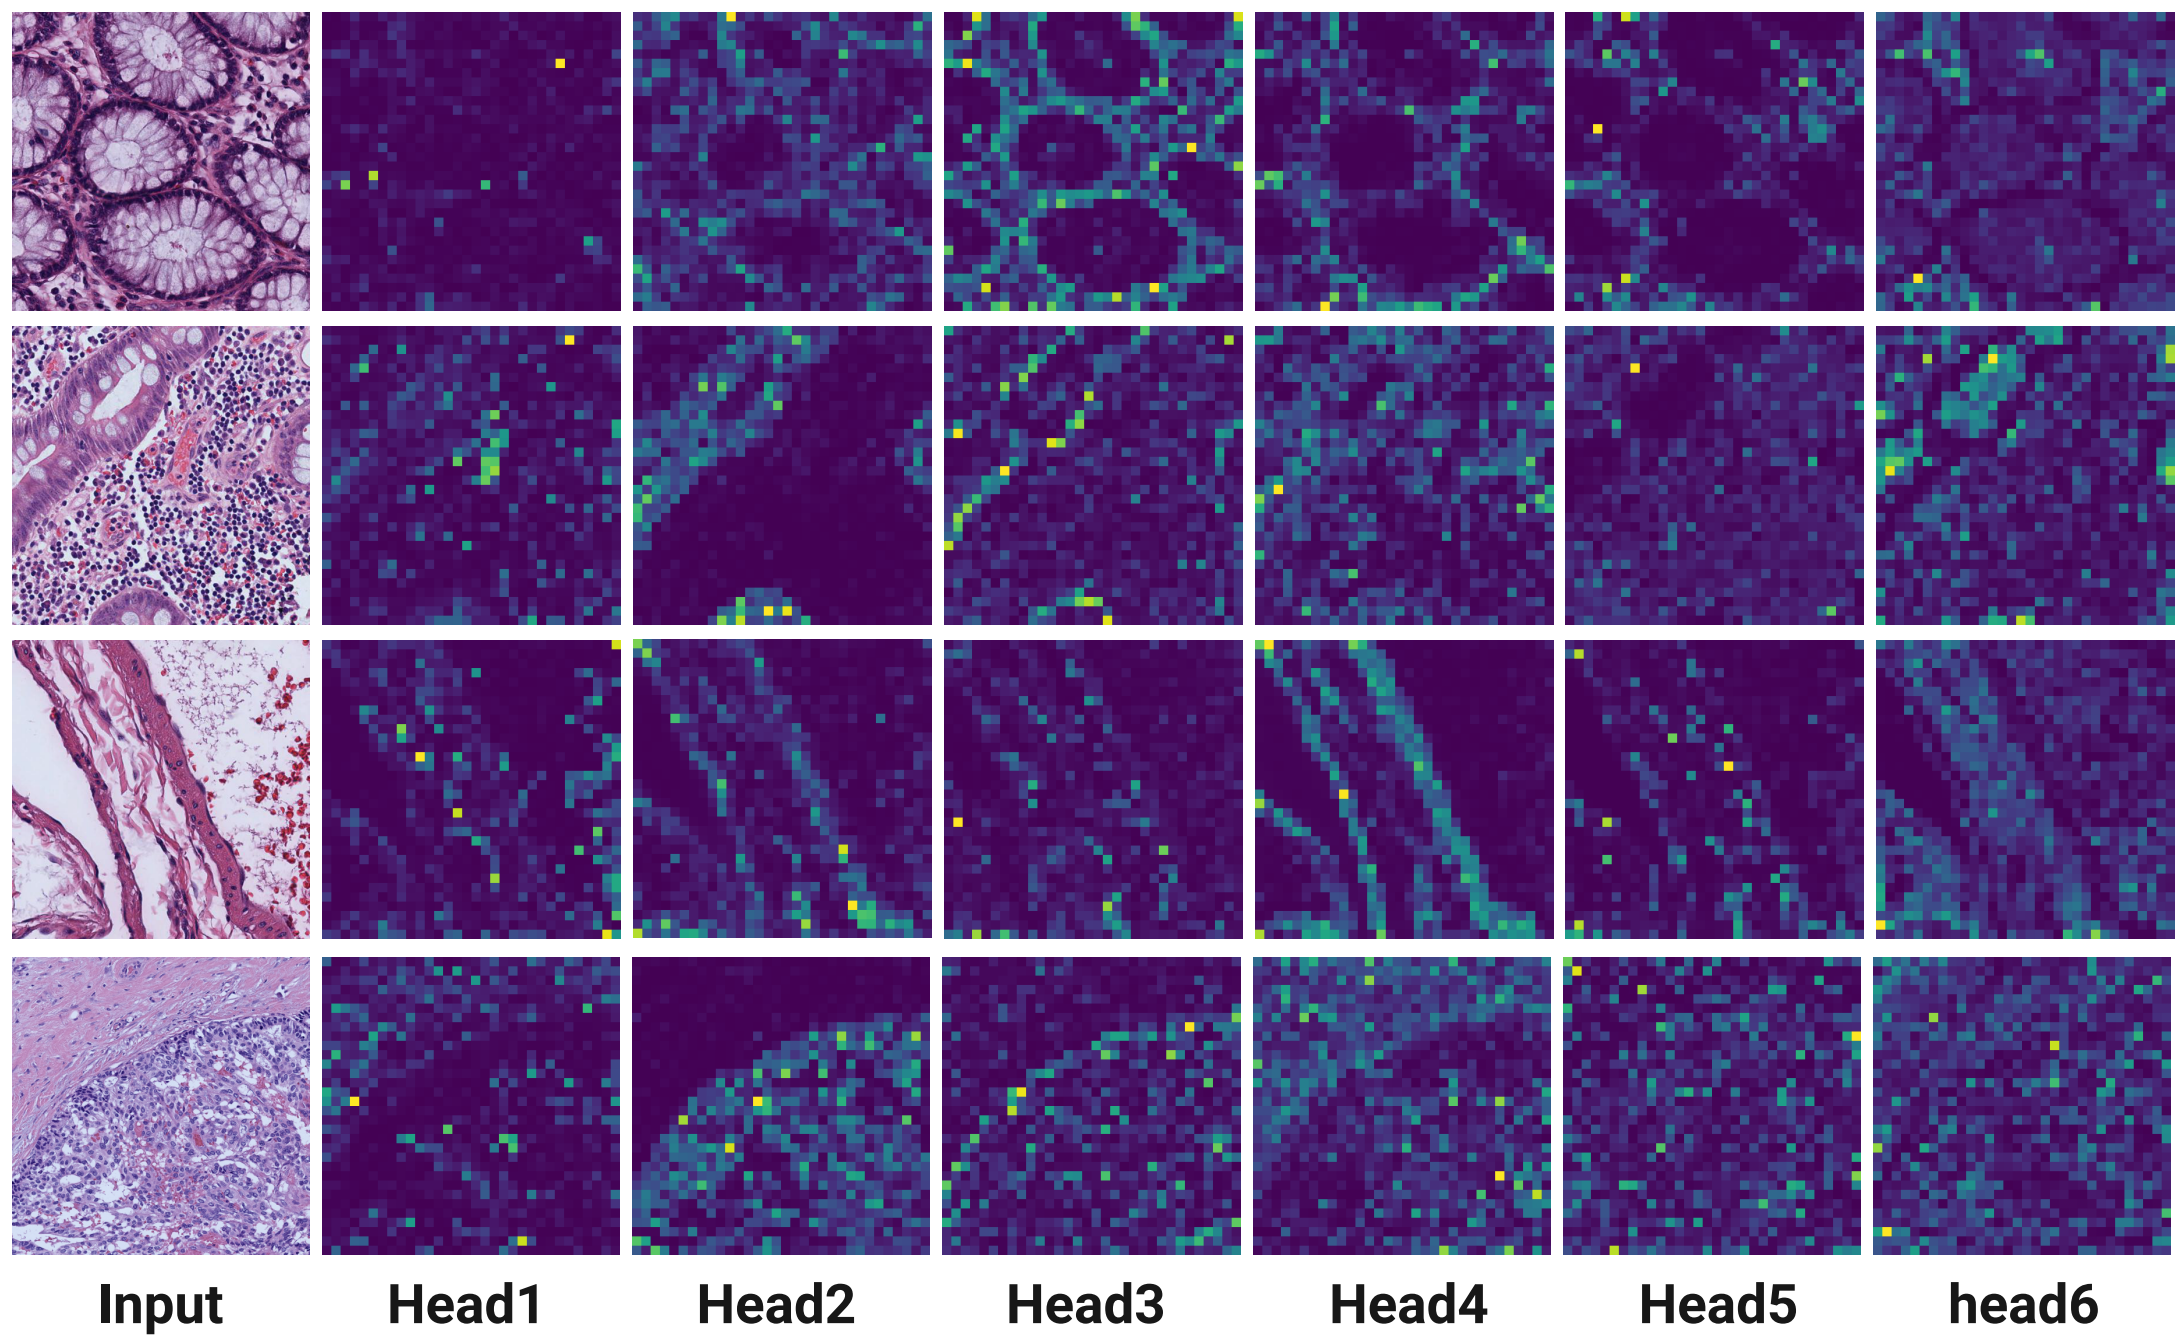



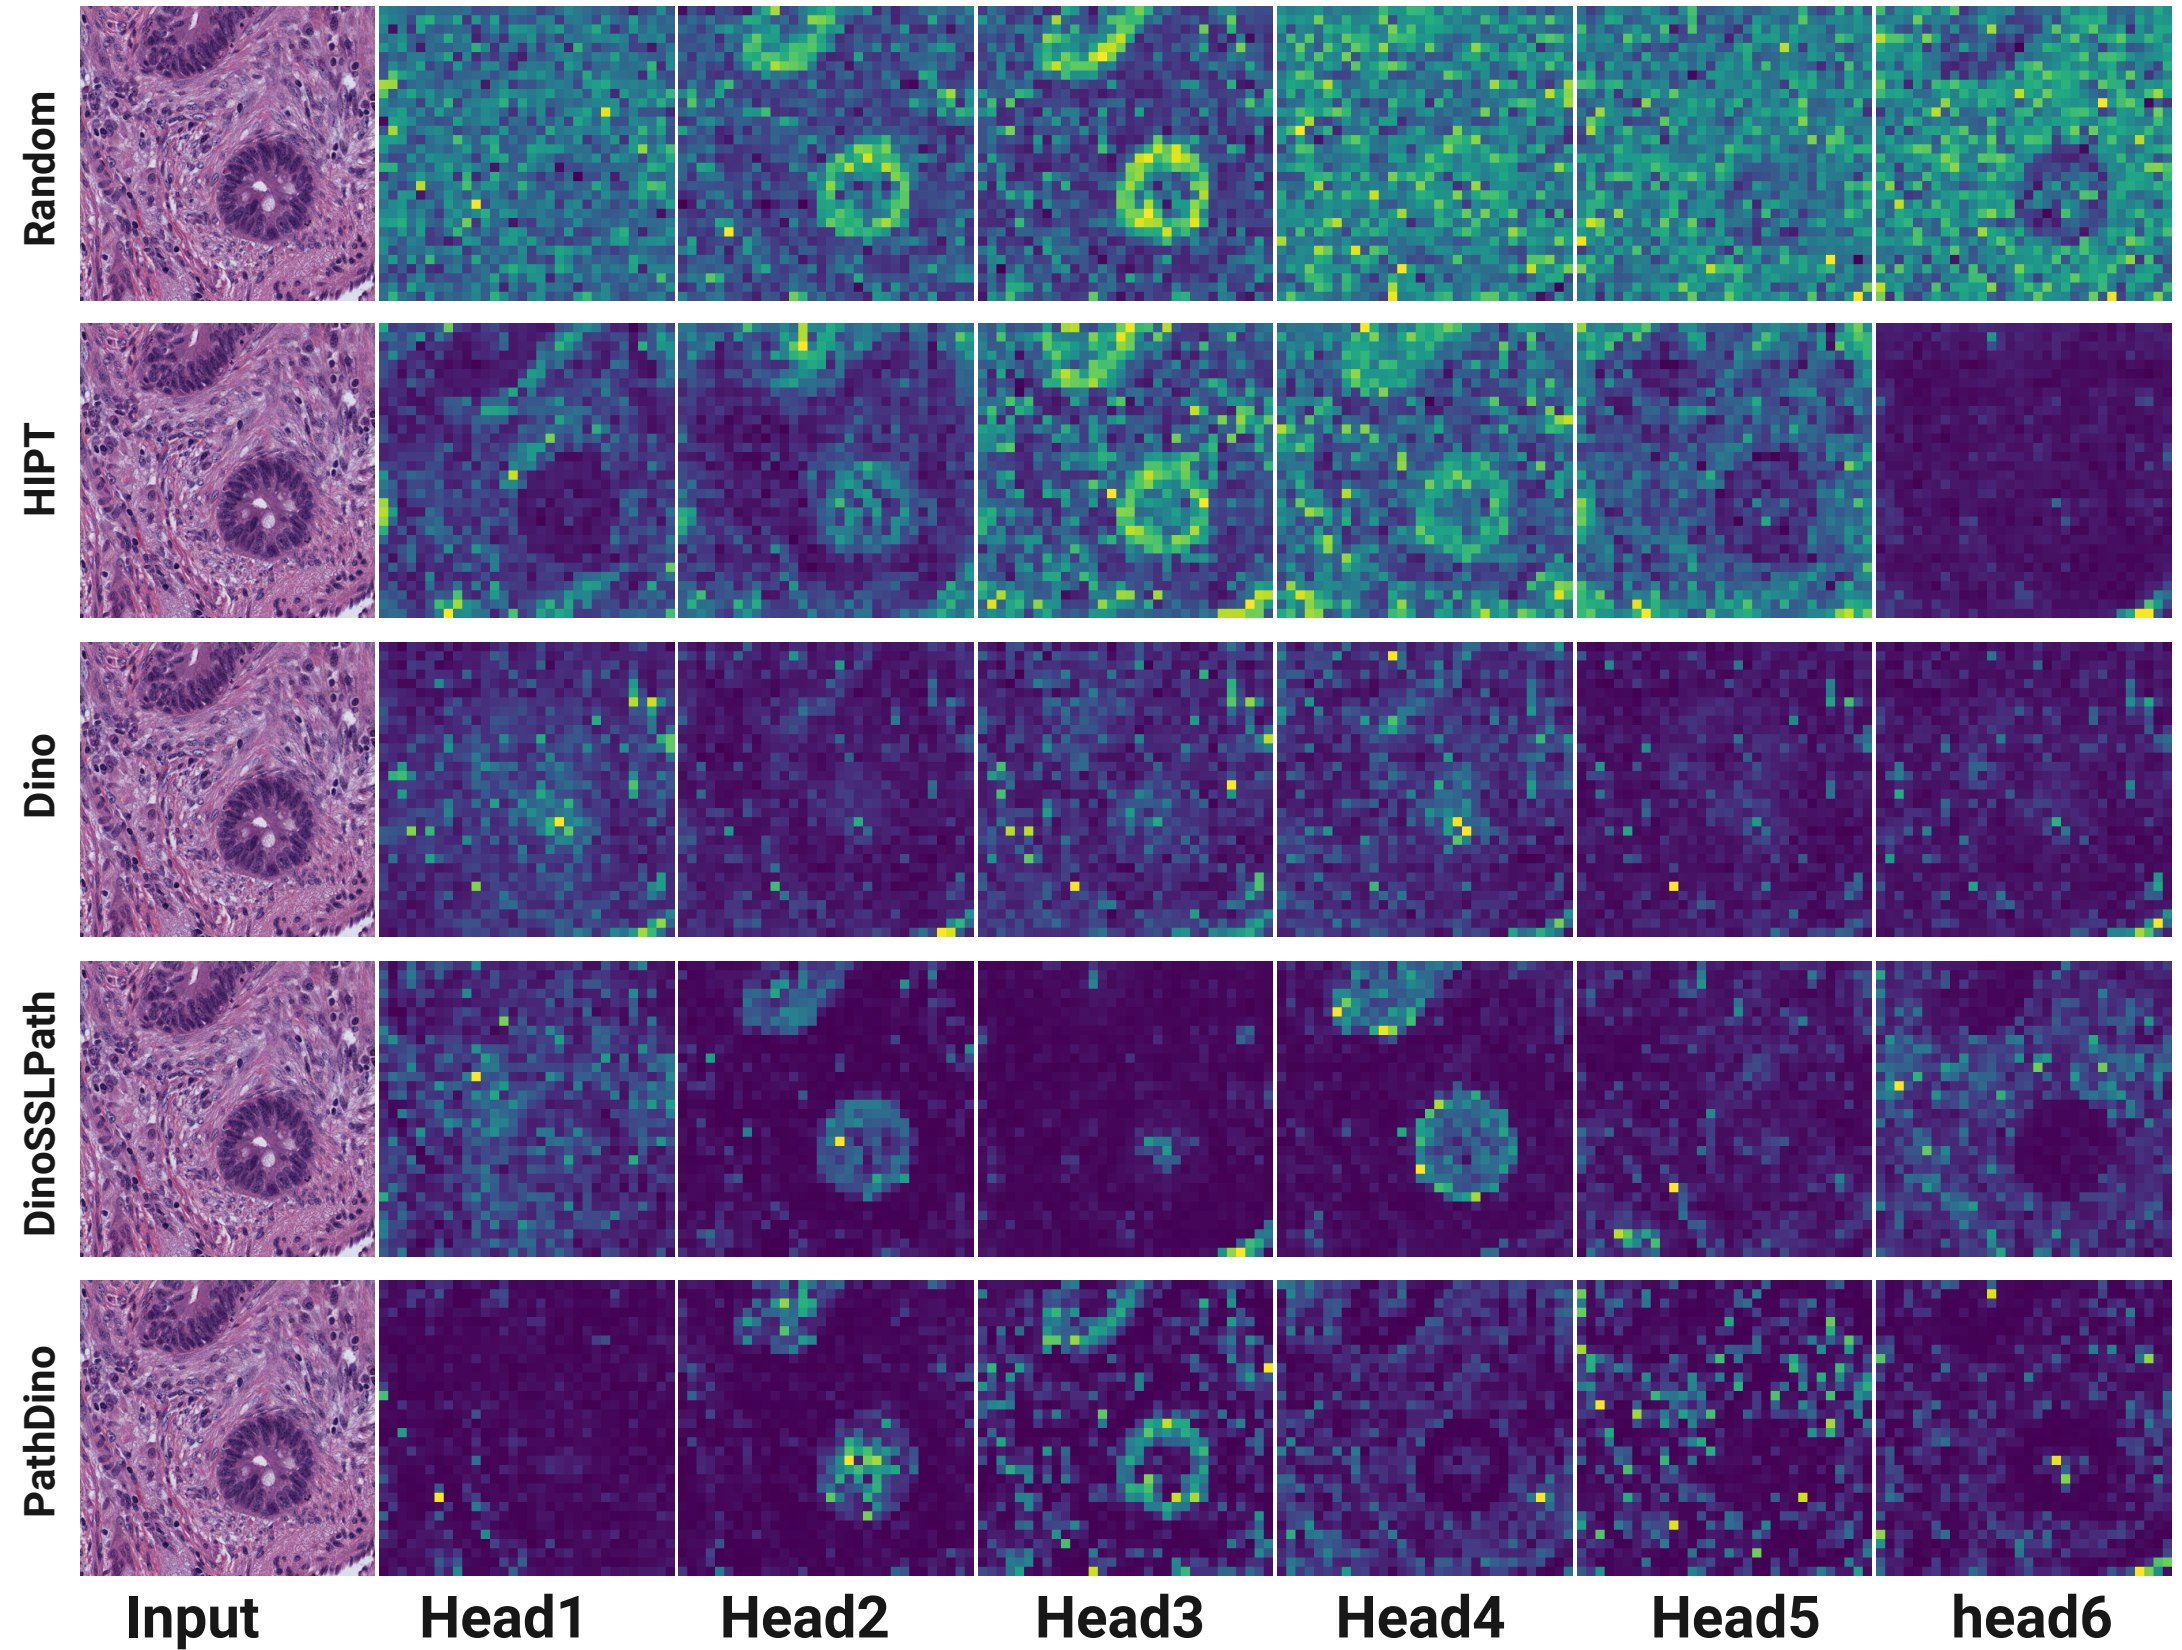

HIPT

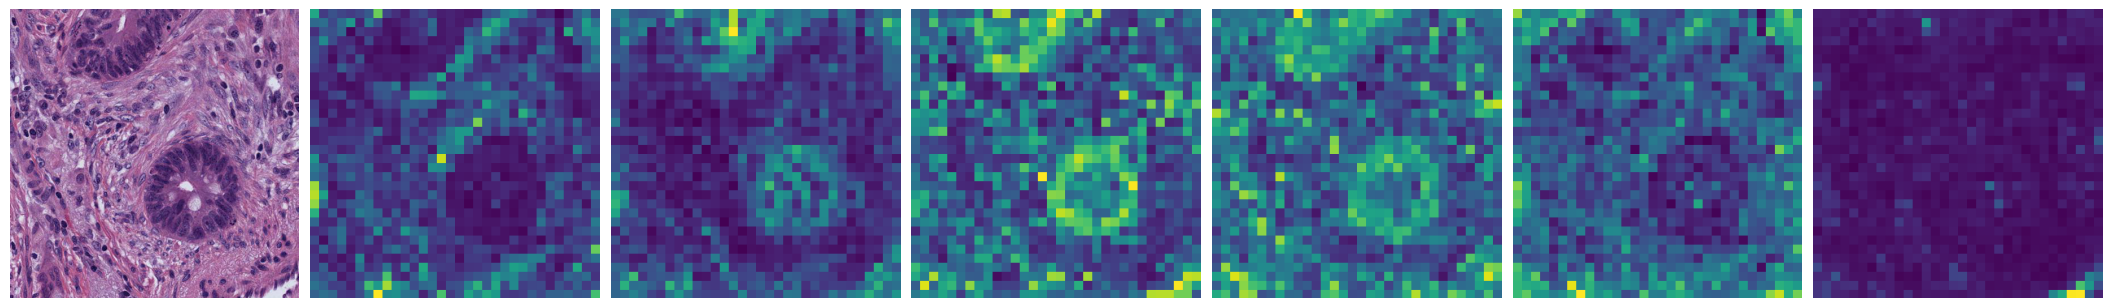

DinoSSLPath

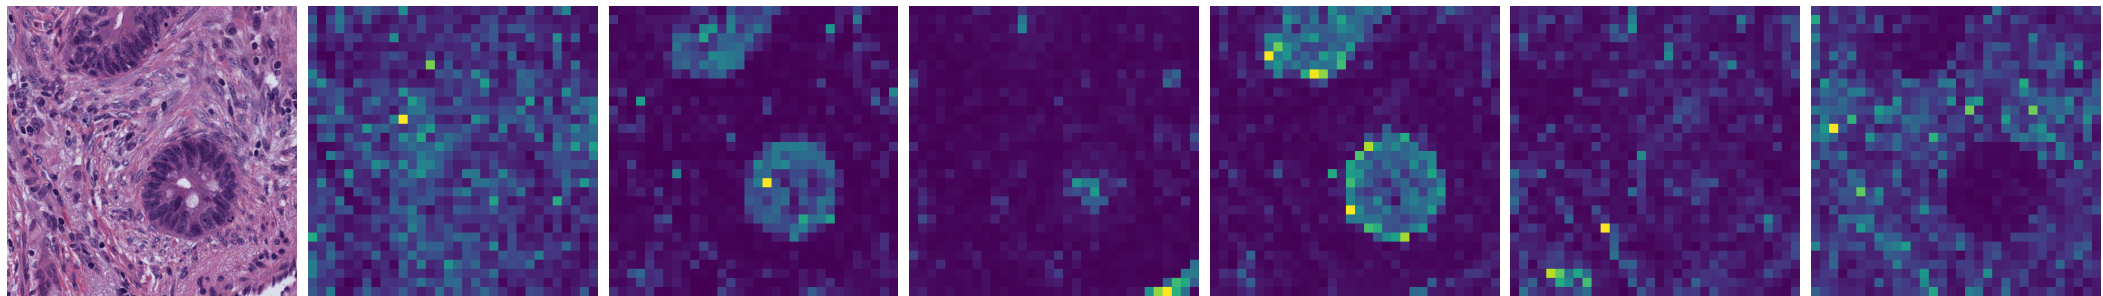

PathDino

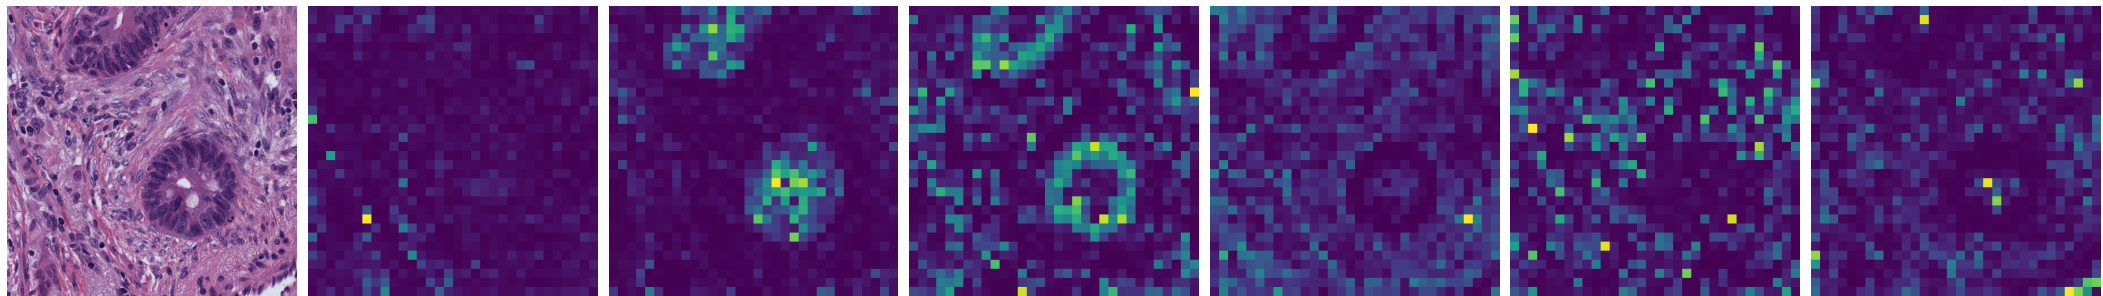

Input

Head1

Head2

Head3

Head4

Head5

head6



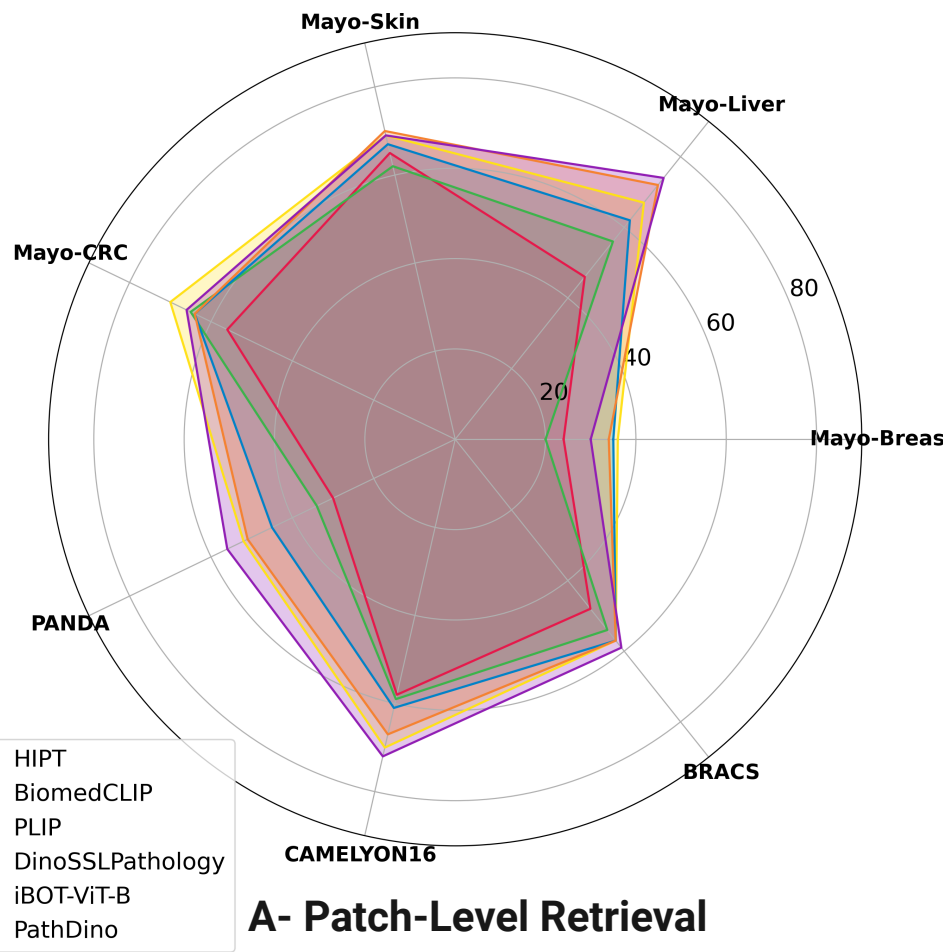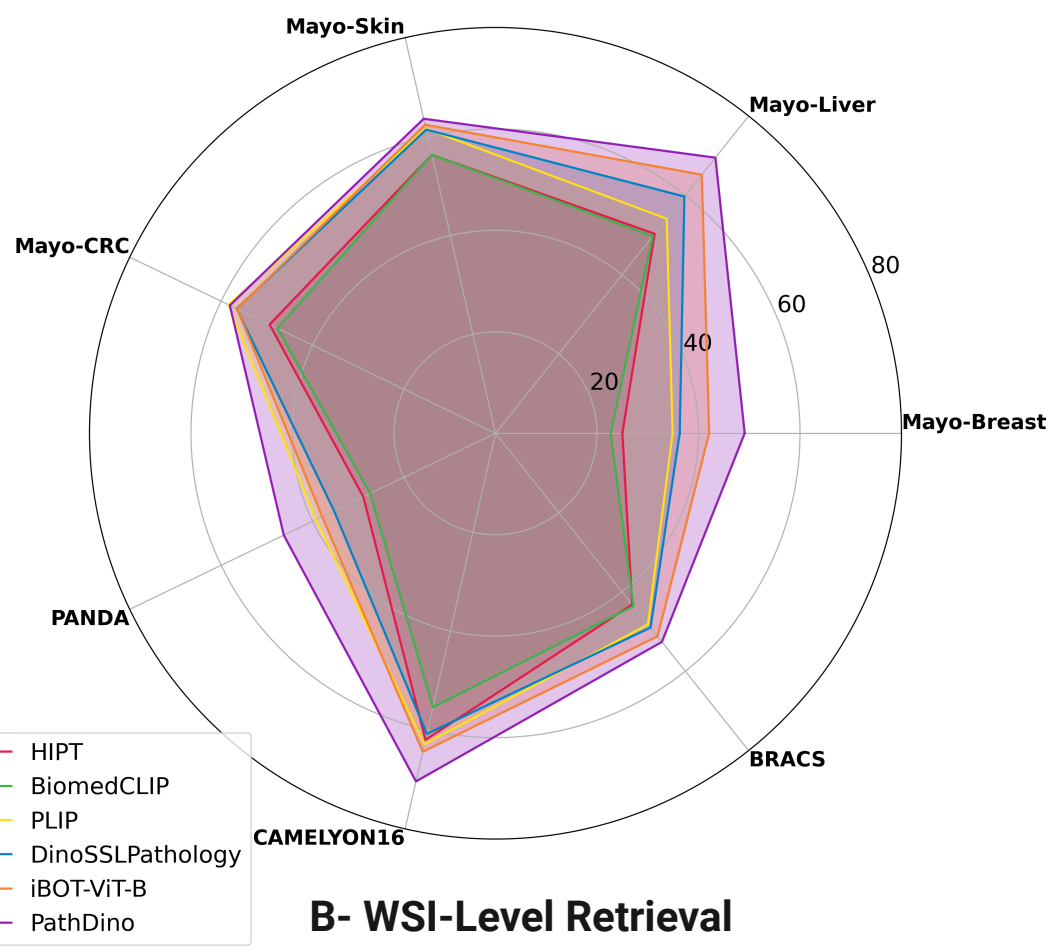

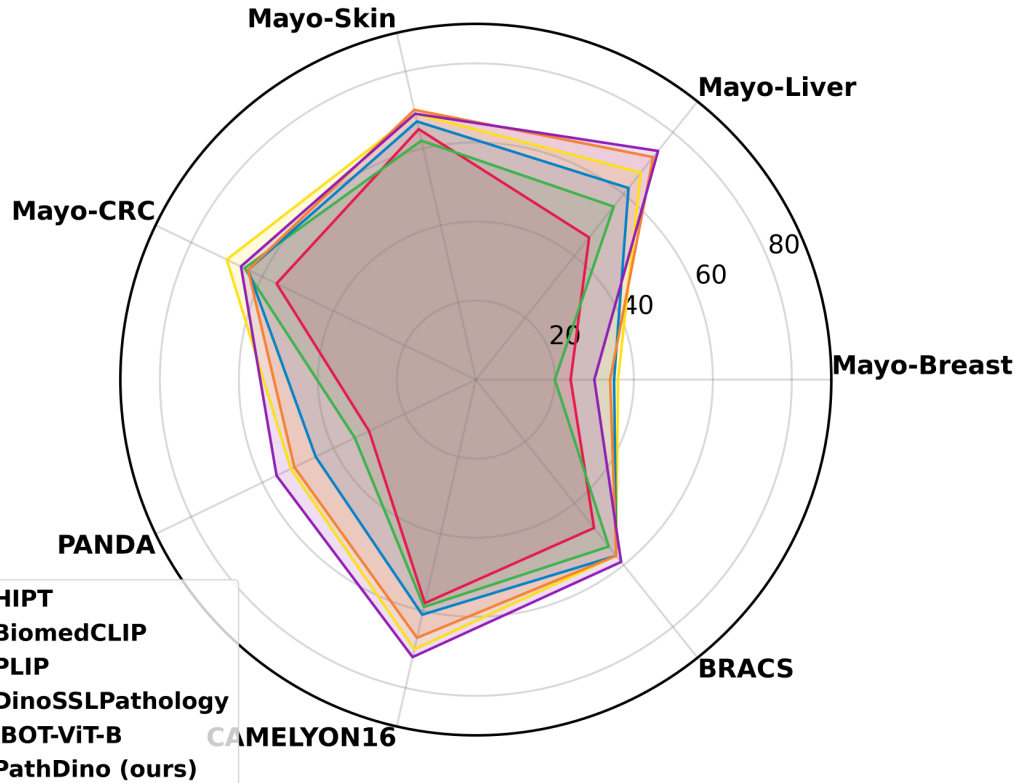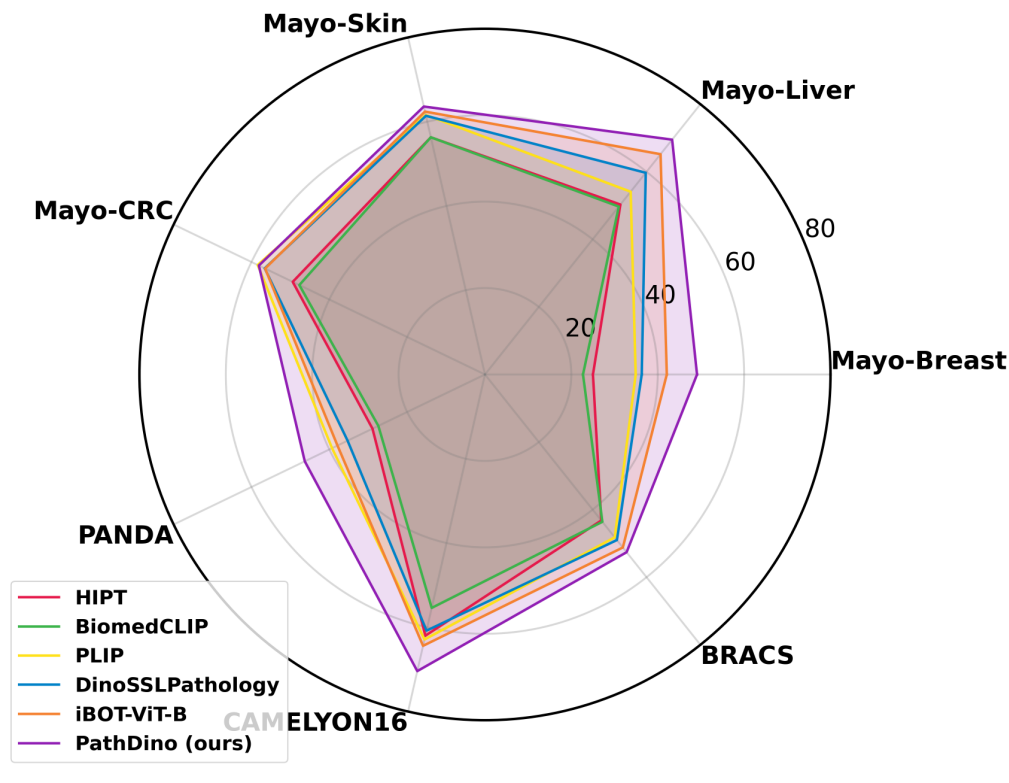

Supplement: Supplementary file 1 [file FigSuppActivationMap.pdf]
